# Supplementary material for: Structural Language Models of Code
Source: arXiv:1910.00577 source file (2020-07-29)
Supplement: Supplementary file 1 [file csharp_appendix_anycode_examples.tex]

%%%%%%%%%%%%%%%%%%%%%%%%%%%%%%%%%%%%%%%%%%%%%%%%%%%%%%%%%%%%%%%%%%%%%%%%%%%%%%%%%%%%%%%

\begin{figure}[t]
\begin{subfigure}[t!]{1.0\textwidth}
\vspace{2mm}
\begin{minted}[fontsize=\footnotesize, frame=single,framesep=2pt,escapeinside=||]{csharp}
public static int TrailingSpaces(this StringBuilder builder)                                                                                                               
{                                                                                                                                                                          
    var bound = builder.Length - 1;                                                                                                                                        
    if (builder.Length == 0) return 0;                                                                                                                                     
    if (builder[bound] != ' ') return 0;                                                                                                                                   
    var c = 0;                                                                                                                                                             
    for (var i = bound; i <= bound; i--)                                                                                                                                   
    {                                                                                                                                                                      
        if (i < 0) break;                                                                                                                                                  
        if (|\greenbox{builder[i]}| != ' ') break;                                                                                                                                      
        c++;                                                                                                                                                               
    }                                                                                                                                                                      
    return c;                                                                                                                                                              
} 
\end{minted}
\end{subfigure}
\\
\vspace{1mm}

\begin{subfigure}[]{0.9\textwidth}
\footnotesize
\centering
\begin{tabular}{|l|lr|}
\hline
\bf{Model}  & \bf{Prediction} &  \\
\hline
True ref:                            & \texttt{builder[i]} & \\
\hline
\multirow{3}{*}{SLM (this work)}             & \texttt{\textbf{builder[i]}} & (62.2\%) \\
                                 & \texttt{c[i]} & (2.6\%) \\
                                 & \texttt{builder.length} & (1.8\%) \\
\hline
\end{tabular}
\vspace{2mm}
\end{subfigure} \\\vspace{2mm}
\noindent\rule{\textwidth}{1pt}

\begin{subfigure}[t!]{1.0\textwidth}
\vspace{2mm}
\begin{minted}[fontsize=\footnotesize, frame=single,framesep=2pt,escapeinside=||]{csharp}
Maybe<Tuple<PropertyInfo, UsageAttribute>> GetUsageData(this Type type)                                                                                      
{                                                                                                                                                                          
    return                                                                                                                                                                 
        (from pi in type.FlattenHierarchy().SelectMany(
                x => x.GetTypeInfo().GetProperties())                                                                               
         let attrs = |\greenbox{pi.GetCustomAttributes}|(true)                                                                                                                       
         where attrs.OfType<UsageAttribute>().Any()                                                                                                                     
         select Tuple.Create(pi, (UsageAttribute)attrs.First()))                                                                                                        
             .SingleOrDefault()                                                                                                                                         
             .ToMaybe();                                                                                                                                                
}
\end{minted}
\end{subfigure}
\\
\vspace{1mm}

\begin{subfigure}[]{0.9\textwidth}
\footnotesize
\centering
\begin{tabular}{|l|lr|}
\hline
\bf{Model}  & \bf{Prediction} &  \\
\hline
True ref:                            & \texttt{pi.GetCustomAttributes} & \\
\hline
\multirow{3}{*}{SLM (this work)}             & \texttt{\textbf{pi.GetCustomAttributes}} & (4.7\%) \\
                                 & \texttt{type.GetInterfaces} & (4.6\%) \\
                                 & \texttt{type.GetFields} & (2.4\%) \\
\hline
\end{tabular}
\end{subfigure} \\\vspace{2mm}

\caption{C\# examples from our test set of the \aeg{} task along with the predictions of our model.}
\label{appendix_csharp_unlimited_figure_intro_example}
\end{figure}

%%%%%%%%%%%%%%%%%%%%%%%%%%%%%%%%%%%%%%%%%%%%%%%%%%%%%%%%%%%%%%%%%%%%%%%%%%%%%%%%%%%%%%%

%%%%%%%%%%%%%%%%%%%%%%%%

\begin{figure}[t]
\begin{subfigure}[t!]{1.0\textwidth}
\vspace{2mm}
\begin{minted}[fontsize=\footnotesize, frame=single,framesep=2pt,escapeinside=||]{csharp}
private string ApplyRules(IList<Rule> rules, string word)                                                                                                                  
{                                                                                                                                                                          
    if (word == null)                                                                                                                                                      
        return null;                                                                                                                                                       
                                                                                                                                                                           
    if (IsUncountable(word))                                                                                                                                               
        return word;                                                                                                                                                       
                                                                                                                                                                           
    var result = word;                                                                                                                                                     
    for (var i = rules.Count - 1; i >= 0; i--)                                                                                                                             
    {                                                                                                                                                                      
        if ((result = |\greenbox{rules[i]}|.Apply(word)) != null)                                                                                                                       
            break;                                                                                                                                                         
    }                                                                                                                                                                      
    return result;                                                                                                                                                         
}    
\end{minted}
\end{subfigure}
\\
\vspace{1mm}

\begin{subfigure}[]{0.9\textwidth}
\footnotesize
\centering
\begin{tabular}{|l|lr|}
\hline
\bf{Model}  & \bf{Prediction} &  \\
\hline
True ref:                            & \texttt{rules[i]} & \\
\hline
\multirow{3}{*}{SLM (this work)}             & \texttt{\textbf{rules[i]}} & (16.8\%) \\
                                 & \texttt{DateTime.UtcNow} & (4.0\%) \\
                                 & \texttt{rules.SelectMany()} & (0.9\%) \\
\hline
\end{tabular}
\vspace{2mm}
\end{subfigure} \\\vspace{2mm}
\noindent\rule{\textwidth}{1pt}

\begin{subfigure}[t!]{1.0\textwidth}
\vspace{2mm}
\begin{minted}[fontsize=\footnotesize, frame=single,framesep=2pt,escapeinside=||]{csharp}
public void SetFilter(
    Func<OptionFilterUniverse, OptionFilterUniverse> universeFunc)
{
    ContractFilter = new FuncSecurityDerivativeFilter(universe =>
    {
        var optionUniverse = universe as OptionFilterUniverse;
        var result = |\greenbox{universeFunc(optionUniverse)}|;
        return result.ApplyOptionTypesFilter();
    });
}
\end{minted}
\end{subfigure}
\\
\vspace{1mm}

\begin{subfigure}[]{0.9\textwidth}
\footnotesize
\centering
\begin{tabular}{|l|lr|}
\hline
\bf{Model}  & \bf{Prediction} &  \\
\hline
True ref:                            & \texttt{universeFunc(optionUniverse)} & \\
\hline
\multirow{3}{*}{SLM (this work)}             & \texttt{\textbf{universeFunc(optionUniverse)}} & (8.7\%) \\
                                 & \texttt{optionUniverse(optionUniverse)} & (5.9\%) \\
                                 & \texttt{optionUniverse as OptionFilterUniverse} & (3.6\%) \\
\hline
\end{tabular}
\end{subfigure} \\\vspace{2mm}

\caption{C\# examples from our test set of the \aeg{} task along with the predictions of our model.}
\label{appendix_csharp_unlimited_figure}
\end{figure}

%%%%%%%%%%%%%%%%%%%%%%%%%%%%%%%%%%%%%%%%%%%%%%%%%%%%%%%%%%%%%%%%%%%%%%%%%%%%%%%%%%%%%%%

%%%%%%%%%%%%%%%%%%%%%%%%

\begin{figure}[t]
\begin{subfigure}[t!]{1.0\textwidth}
\vspace{2mm}
\begin{minted}[fontsize=\footnotesize, frame=single,framesep=2pt,escapeinside=||]{csharp}
private OrderDirection ConvertOrderDirection(string direction)
{
    switch (direction)
    {
        case IB.ActionSide.Buy: return OrderDirection.Buy;
        case IB.ActionSide.Sell: return |\greenbox{OrderDirection.Sell}|;
        case IB.ActionSide.Undefined: return OrderDirection.Hold;
        default:
            throw new ArgumentException(direction, "direction");
    }
}
\end{minted}
\end{subfigure}
\\
\vspace{1mm}

\begin{subfigure}[]{0.9\textwidth}
\footnotesize
\centering
\begin{tabular}{|l|lr|}
\hline
\bf{Model}  & \bf{Prediction} &  \\
\hline
True ref:                            & \texttt{OrderDirection.Sell} & \\
\hline
\multirow{3}{*}{SLM (this work)}             & \texttt{\textbf{OrderDirection.Sell}} & (61.5\%) \\
                                 & \texttt{IB.Sell.Sell} & (12.5\%) \\
                                 & \texttt{IB.ActionSide.Sell} & (4.4\%) \\
\hline
\end{tabular}
\vspace{2mm}
\end{subfigure} \\\vspace{2mm}
\noindent\rule{\textwidth}{1pt}

\begin{subfigure}[t!]{1.0\textwidth}
\vspace{2mm}
\begin{minted}[fontsize=\footnotesize, frame=single,framesep=2pt,escapeinside=||]{csharp}
public void StartSession()
{
    _shutdown = false;

    _response = GetSession();

    _runningTask = Task.Run(() =>
    {
        using (var reader = 
            new StreamReader(_response.GetResponseStream()))
        {
            while (!_shutdown)
            {
                var line = |\greenbox{reader.ReadLine()}|;

                var handler = DataReceived;
                if (handler != null) handler(line);
            }
        }
    });
}
\end{minted}
\end{subfigure}
\\
\vspace{1mm}

\begin{subfigure}[]{0.9\textwidth}
\footnotesize
\centering
\begin{tabular}{|l|lr|}
\hline
\bf{Model}  & \bf{Prediction} &  \\
\hline
True ref:                            & \texttt{reader.ReadLine()} & \\
\hline
\multirow{3}{*}{SLM (this work)}             & \texttt{\textbf{reader.ReadLine()}} & (45.6\%) \\
                                 & \texttt{reader.ReadLine()()} & (2.3\%) \\
                                 & \texttt{getLine()} & (1.0\%) \\
\hline
\end{tabular}
\vspace{2mm}
\end{subfigure} \\\vspace{2mm}

\caption{C\# examples from our test set of the \aeg{} task along with the predictions of our model.}
\label{appendix_csharp_unlimited_figure}
\end{figure}

%%%%%%%%%%%%%%%%%%%%%%%%%%%%%%%%%%%%%%%%%%%%%%%%%%%%%%%%%%%%%%%%%%%%%%%%%%%%%%%%%%%%%%%

%%%%%%%%%%%%%%%%%%%%%%%%

\begin{figure}[t]
\begin{subfigure}[t!]{1.0\textwidth}
\vspace{2mm}
\begin{minted}[fontsize=\footnotesize, frame=single,framesep=2pt,escapeinside=||]{csharp}
private static string FindIndexedProcessName(int pid)
{
    var processName = Process.GetProcessById(pid).ProcessName;
    var processesByName = Process.GetProcessesByName(processName);
    string processIndexdName = null;

    for (var index = 0;  |\greenbox{index < processesByName.Length}| ; index++)
    {
        processIndexdName = 
            index == 0 ? processName : processName + "#" + index;
        var processId = new PerformanceCounter(
            "Process", "ID Process", processIndexdName);
        if ((int)processId.NextValue() == pid)
        {
            return processIndexdName;
        }
    }

    return processIndexdName;
}
\end{minted}
\end{subfigure}
\\
\vspace{1mm}

\begin{subfigure}[]{0.9\textwidth}
\footnotesize
\centering
\begin{tabular}{|l|lr|}
\hline
\bf{Model}  & \bf{Prediction} &  \\
\hline
True ref:                            & \texttt{index < processesByName.Length} & \\
\hline
\multirow{3}{*}{SLM (this work)}             & \texttt{\textbf{index < processesByName.Length}} & (12.8\%) \\
                                 & \texttt{indexOf < processesByName.Length} & (6.1\%) \\
                                 & \texttt{index < processesByName} & (4.0\%) \\
\hline
\end{tabular}
\vspace{2mm}
\end{subfigure} \\\vspace{2mm}
\noindent\rule{\textwidth}{1pt}

\begin{subfigure}[t!]{1.0\textwidth}
\vspace{2mm}
\begin{minted}[fontsize=\footnotesize, frame=single,framesep=2pt,escapeinside=||]{csharp}
private static Stream GetResponseStream(WebResponse response)
{
    var stream = |\greenbox{response.GetResponseStream()}|;
    if (response.Headers["Content-Encoding"] == "gzip")
    {
        // if we received a gzipped response, handle that
        if (stream != null) 
            stream = new GZipStream(stream, CompressionMode.Decompress);
    }
    return stream;
}
\end{minted}
\end{subfigure}
\\
\vspace{1mm}

\begin{subfigure}[]{0.9\textwidth}
\footnotesize
\centering
\begin{tabular}{|l|lr|}
\hline
\bf{Model}  & \bf{Prediction} &  \\
\hline
True ref:                            & \texttt{response.GetResponseStream()} & \\
\hline
\multirow{3}{*}{SLM (this work)}             & \texttt{\textbf{response.GetResponseStream()}} & (18.9\%) \\
                                 & \texttt{new Response()} & (6.8\%) \\
                                 & \texttt{new MemoryStream()} & (6.3\%) \\
\hline
\end{tabular}
\end{subfigure} \\\vspace{2mm}

\caption{C\# examples from our test set of the \aeg{} task along with the predictions of our model.}
\label{appendix_csharp_unlimited_figure}
\end{figure}

%%%%%%%%%%%%%%%%%%%%%%%%%%%%%%%%%%%%%%%%%%%%%%%%%%%%%%%%%%%%%%%%%%%%%%%%%%%%%%%%%%%%%%%

%%%%%%%%%%%%%%%%%%%%%%%%

\begin{figure}[t]
\begin{subfigure}[t!]{1.0\textwidth}
\vspace{2mm}
\begin{minted}[fontsize=\footnotesize, frame=single,framesep=2pt,escapeinside=||]{csharp}
public virtual void OnData(Slice slice)
{
    // as a default implementation, let's look for and call OnData(Slice)
    // ... just in case a user forgot to use the override keyword
    if (!_checkedForOnDataSlice)
    {
        _checkedForOnDataSlice = true;
        
        var method = GetType().GetMethods()
            .Where(x => x.Name == "OnData")
            .Where(x => x.DeclaringType != typeof(QCAlgorithm))
            .Where(x => x.GetParameters().Length == 1)
            .FirstOrDefault(
                x => x.GetParameters()[0]
                    .ParameterType == typeof (Slice));

        if (method == null)
        {
            return;
        }

        var self = Expression.Constant(this);
        var parameter = Expression.Parameter(typeof (Slice), "data");
        var call = Expression.Call(self, method, parameter);
        var lambda = Expression.Lambda<Action<Slice>>(call, parameter);
        _onDataSlice = |\greenbox{lambda.Compile()}|;
    }
    // if we have it, then invoke it
    if (_onDataSlice != null)
    {
        _onDataSlice(slice);
    }
}
\end{minted}
\end{subfigure}
\\
\vspace{1mm}

\begin{subfigure}[]{0.9\textwidth}
\footnotesize
\centering
\begin{tabular}{|l|lr|}
\hline
\bf{Model}  & \bf{Prediction} &  \\
\hline
True ref:                            & \texttt{lambda.Compile()} & \\
\hline
\multirow{3}{*}{SLM (this work)}             & \texttt{\textbf{lambda.Compile()}} & (8.5\%) \\
                                 & \texttt{lambda().Compile()} & (4.4\%) \\
                                 & \texttt{!\_checkedForOnDataDataSlice} & (3.4\%) \\
\hline
\end{tabular}
\end{subfigure}

\vspace{2mm}
\noindent\rule{\textwidth}{1pt}

\begin{subfigure}[t!]{1.0\textwidth}
\vspace{2mm}
\begin{minted}[fontsize=\footnotesize, frame=single,framesep=2pt,escapeinside=||]{csharp}
private void HandleBrokerTime(object sender, IB.CurrentTimeUtcEventArgs e)
{
    // keep track of clock drift
    _brokerTimeDiff = e.CurrentTimeUtc.Subtract(|\greenbox{DateTime.UtcNow}|);
}
\end{minted}
\end{subfigure}
\\
\vspace{1mm}

\begin{subfigure}[]{0.9\textwidth}
\footnotesize
\centering
\begin{tabular}{|l|lr|}
\hline
\bf{Model}  & \bf{Prediction} &  \\
\hline
True ref:                            & \texttt{DateTime.UtcNow} & \\
\hline
\multirow{3}{*}{SLM (this work)}             & \texttt{\textbf{DateTime.UtcNow}} & (28.1\%) \\
                                 & \texttt{TimeSpan.Zero} & (6.9\%) \\
                                 & \texttt{CurrentTimeUtcEventArgs.Broker} & (2.6\%) \\
\hline
\end{tabular}
\end{subfigure} 

\caption{C\# examples from our test set of the \aeg{} task along with the predictions of our model.}
\label{appendix_csharp_unlimited_figure}
\end{figure}

%%%%%%%%%%%%%%%%%%%%%%%%%%%%%%%%%%%%%%%%%%%%%%%%%%%%%%%%%%%%%%%%%%%%%%%%%%%%%%%%%%%%%%%
